# Supplementary material for: Learning Gaussian Mixtures Using the Wasserstein-Fisher-Rao Gradient Flow
Source: arXiv:2301.01766 source file (2023-01-04)
Supplement: Supplementary file 1 [file appendix_BW.tex]

\section{Proof of Theorem XXX (BW)}

We first compute the first variation $\delta\mathcal{L}(\rho):\Theta\to\mathbb{R}$
of the negative log-likelihood functional 
\[
\mathcal{L}\left(\rho\right)=-\frac{1}{N}\sum_{i=1}^{N}\log\int\phi\left(X_{i};\theta\right)\rho\left(\mathrm{d}\theta\right).
\]
For any $\varepsilon>0$ and any measure $\mathcal{X}$ satisfying
$\int_{\Theta}\mathrm{d}\mathcal{X}=0$, we have
\begin{align*}
\lim_{\varepsilon\to0}\frac{1}{\varepsilon}\left[\mathcal{L}\left(\rho+\varepsilon\mathcal{X}\right)-\mathcal{L}\left(\rho\right)\right] & =-\frac{1}{N}\sum_{i=1}^{N}\lim_{\varepsilon\to0}\frac{1}{\varepsilon}\left[\log\int\phi\left(X_{i};\theta\right)\left(\rho+\varepsilon\mathcal{X}\right)\left(\mathrm{d}\theta\right)-\log\int\phi\left(X_{i};\theta\right)\rho\left(\mathrm{d}\theta\right)\right]\\
 & =-\frac{1}{N}\sum_{i=1}^{N}\lim_{\varepsilon\to0}\frac{1}{\varepsilon}\log\left[1+\varepsilon\frac{\int\phi\left(X_{i};\theta\right)\mathcal{X}\left(\mathrm{d}\theta\right)}{\int\phi\left(X_{i};\theta\right)\rho\left(\mathrm{d}\theta\right)}\right]\\
 & =-\frac{1}{N}\sum_{i=1}^{N}\frac{\int\phi\left(X_{i};\theta\right)\mathcal{X}\left(\mathrm{d}\theta\right)}{\int\phi\left(X_{i};\theta\right)\rho\left(\mathrm{d}\theta\right)}.
\end{align*}
By definition, we have
\[
\lim_{\varepsilon\to0}\frac{1}{\varepsilon}\left[\mathcal{L}\left(\rho+\varepsilon\mathcal{X}\right)-\mathcal{L}\left(\rho\right)\right]=\int\delta\ell\left(\rho\right)\left(\theta\right)\mathcal{X}\left(\mathrm{d}\theta\right).
\]
As a result, we can identify the first variation as
\[
\delta\mathcal{L}\left(\rho\right):\theta\to-\frac{1}{N}\sum_{i=1}^{N}\frac{\phi\left(X_{i};\theta\right)}{\int\phi\left(X_{i};\zeta\right)\rho\left(\mathrm{d}\zeta\right)}.
\]
Note that
\begin{align*}
\nabla_{\mu}\delta\mathcal{L}\left(\rho\right)\left(\theta\right) & =-\frac{1}{N}\sum_{i=1}^{N}\frac{\nabla_{\mu}\phi\left(X_{i};\mu,\Sigma\right)}{\int\phi\left(X_{i};\zeta\right)\rho\left(\mathrm{d}\zeta\right)}=-\frac{1}{N}\sum_{i=1}^{N}\frac{\phi\left(X_{i};\mu,\Sigma\right)}{\int\phi\left(X_{i};\zeta\right)\rho\left(\mathrm{d}\zeta\right)}\Sigma^{-1}\left(X_{i}-\mu\right)
\end{align*}
and
\begin{align*}
\nabla_{\Sigma}\delta\mathcal{L}\left(\rho\right)\left(\theta\right) & =-\frac{1}{N}\sum_{i=1}^{N}\frac{\nabla_{\Sigma}\phi\left(X_{i};m,\Sigma\right)}{\int\phi\left(X_{i};\zeta\right)\rho\left(\mathrm{d}\zeta\right)}\\
 & =-\frac{1}{2N}\sum_{i=1}^{N}\frac{\phi\left(X_{i};m,\Sigma\right)}{\int\phi\left(X_{i};\zeta\right)\rho\left(\mathrm{d}\zeta\right)}\left[\Sigma^{-1}\left(X_{i}-\mu\right)\left(X_{i}-\mu\right)^{\top}\Sigma^{-1}-\Sigma^{-1}\right].
\end{align*}
In view of \cite[Section F]{lambert2022variational}, we know that
by equipping $\mathcal{P}_{2}(\Theta)$ with the Wasserstein distance,
the Wasserstein gradient of $\mathcal{F}$ is
\begin{align*}
\nabla_{\mathsf{W}}\mathcal{F}\left(\rho\right)\left(\mu,\Sigma\right) & =\left[\begin{array}{c}
\nabla_{\mu}\delta\mathcal{L}\left(\rho\right)\left(\theta\right)\\
2\nabla_{\Sigma}\delta\mathcal{L}\left(\rho\right)\left(\theta\right)
\end{array}\right]\\
 & =-\frac{1}{N}\sum_{i=1}^{N}\frac{\phi\left(X_{i};\mu,\Sigma\right)}{\int\phi\left(X_{i};\zeta\right)\rho\left(\mathrm{d}\zeta\right)}\left[\begin{array}{c}
\Sigma^{-1}\left(X_{i}-\mu\right)\\
\Sigma^{-1}\left(X_{i}-\mu\right)\left(X_{i}-\mu\right)^{\top}\Sigma^{-1}-\Sigma^{-1}
\end{array}\right].
\end{align*}
In view of \cite[Section H.2]{lambert2022variational}, we know that
the Wasserstein-Fisher-Rao gradient of $\mathcal{F}$ is
\begin{align*}
\nabla_{\mathsf{WFR}}\mathcal{F}\left(\rho\right)\left(\mu,\Sigma\right) & =\left[\begin{array}{c}
\nabla_{\mathsf{BW}}\mathcal{F}\left(\rho\right)\left(\mu,\Sigma\right)\\
\delta\mathcal{L}\left(\rho\right)-\int\delta\mathcal{L}\left(\rho\right)\mathrm{d}\rho
\end{array}\right]\\
 & =-\frac{1}{N}\sum_{i=1}^{N}\frac{\phi\left(X_{i};\mu,\Sigma\right)}{\int\phi\left(X_{i};\zeta\right)\rho\left(\mathrm{d}\zeta\right)}\left[\begin{array}{c}
\Sigma^{-1}\left(X_{i}-\mu\right)\\
\Sigma^{-1}\left(X_{i}-\mu\right)\left(X_{i}-\mu\right)^{\top}\Sigma^{-1}-\Sigma^{-1}\\
1
\end{array}\right]+\left[\begin{array}{c}
0\\
0\\
1
\end{array}\right].
\end{align*}
Then we know that the following ODE system describes the evolution
of $\{\rho_{t}\}_{t\geq0}$
\begin{align*}
\dot{\mu}_{t} & =\frac{1}{N}\sum_{i=1}^{N}\frac{\phi\left(X_{i};\mu_{t},\Sigma_{t}\right)}{\int\phi\left(X_{i};\zeta\right)\rho_{t}\left(\mathrm{d}\zeta\right)}\Sigma_{t}^{-1}\left(X_{i}-\mu_{t}\right),\\
\dot{\Sigma}_{t} & =\frac{1}{N}\sum_{i=1}^{N}\frac{\phi\left(X_{i};m_{t},\Sigma_{t}\right)}{\int\phi\left(X_{i};\zeta\right)\rho_{t}\left(\mathrm{d}\zeta\right)}\left[\left(X_{i}-\mu_{t}\right)\left(X_{i}-\mu_{t}\right)^{\top}\Sigma_{t}^{-1}+\Sigma_{t}^{-1}\left(X_{i}-\mu_{t}\right)\left(X_{i}-\mu_{t}\right)^{\top}-2I\right],\\
\dot{r}_{t} & =\left[\frac{1}{N}\sum_{i=1}^{N}\frac{\phi\left(X_{i};\mu,\Sigma\right)}{\int\phi\left(X_{i};\zeta\right)\rho\left(\mathrm{d}\zeta\right)}-1\right]r_{t}.
\end{align*}
